# Supplementary material for: On Bell's dynamical route to special relativity
Source: arXiv:2506.23450 source file (2025-06-30)
Supplement: Supplementary file 1 [file ajp_supplemental.pdf]

# Supplemental Information for "On Bell's Dynamical Route to Special Relativity"

Frederick W. Strauch
(Dated: January 18, 2024)

## I. EQUATION OF MOTION FOR AN ELECTRON ORBITING AN ACCELERATED NUCLEUS

The equation of motion for an electron,

$$\frac{d}{dt}\left(\frac{m\mathbf{u}}{\sqrt{1-u^2/c^2}}\right) = -e\left(\mathbf{E} + \mathbf{u}\times\mathbf{B}\right), \tag{1}$$

when the nucleus is in arbitrary motion, requires the full electric and magnetic fields

$$\mathbf{E}(\mathbf{r},t) = \frac{q}{4\pi\epsilon_0}\frac{R}{(\mathbf{R}\cdot\mathbf{U})^3}\left[(c^2-v^2)\mathbf{U} + \mathbf{R}\times(\mathbf{U}\times\mathbf{a})\right] \tag{2}$$

and

$$\mathbf{B}(\mathbf{r},t) = \frac{1}{c}\hat{\mathbf{R}}\times\mathbf{E}(\mathbf{r},t). \tag{3}$$

Here $\mathbf{R} = \mathbf{r} - \mathbf{r}_n(t_r)$, where $\mathbf{r}_n(t)$ is the position of the nucleus, $\mathbf{U} = c\hat{\mathbf{R}} - \mathbf{v}$, $t_r = t - R/c$ is the retarded time, and the velocity $\mathbf{v} = d\mathbf{r}_n/dt$ and the acceleration $\mathbf{a} = d^2\mathbf{r}_n/dt^2$ are evaluated at time $t_r$.

For the orbital contraction problem considered in the text, I let the trajectory of the nucleus be $\mathbf{r}_n = (x_n, 0)$, where

$$x_n(t) = \begin{cases} x_0 & \text{for } t < 0, \\ \sqrt{x_0^2 + c^2t^2} & \text{for } t > 0. \end{cases} \tag{4}$$

For this trajectory one can calculate an explicit expression for the retarded time $t_r$ as a function of $t$ and $\mathbf{r} = (x, y)$:

$$t_r = \begin{cases} \frac{1}{2}\frac{(c^2t^2-r^2-x_0^2)}{(c^2t^2-x^2)}t + \frac{1}{2}\frac{x/c}{(c^2t^2-x^2)}\left[(c^2t^2-r^2-x_0)^2 + 4x_0^2(c^2t^2-x^2)\right]^{1/2} & \text{for } t > \sqrt{(x-x_0)^2+y^2}/c, \\ t - \sqrt{(x-x_0)^2+y^2}/c & \text{for } t < \sqrt{(x-x_0)^2+y^2}/c. \end{cases} \tag{5}$$

To complete the expressions for the electric and magnetic fields, one needs $\mathbf{v} = (v, 0)$, where

$$v = \left(\frac{dx_n}{dt}\right)_{t=t_r} = \begin{cases} 0 & \text{for } t_r < 0, \\ c^2t_r(x_0^2 + c^2t_r^2)^{-1/2} & \text{for } t_r > 0, \end{cases} \tag{6}$$

and $\mathbf{a} = (a, 0)$, where

$$a = \left(\frac{dv}{dt}\right)_{t=t_r} = \begin{cases} 0 & \text{for } t_r < 0, \\ c^2x_0^2(x_0^2 + c^2t_r^2)^{-3/2} & \text{for } t_r > 0, \end{cases} \tag{7}$$

Evaluating the various vector products for this trajectory yields the final results

$$\begin{aligned} E_x(x,y,t) &= E_0\frac{r_0^2}{[R-(v/c)(x-x_n)]^3}\left[(1-v^2/c^2)(x-x_n-Rv/c) - y^2a/c^2\right], \\ E_y(x,y,t) &= E_0\frac{r_0^2}{[R-(v/c)(x-x_n)]^3}\left[(1-v^2/c^2)y + (x-x_n)ya/c^2\right], \\ B_z(x,y,t) &= \frac{E_0}{c}\frac{r_0^2}{[R-(v/c)(x-x_n)]^3}y\left[(1-v^2/c^2)(v/c) + Ra/c^2\right], \end{aligned} \tag{8}$$

where $E_0 = q/(4\pi\epsilon_0 r_0^2)$ and $R = \sqrt{(x-x_n)^2 + y^2}$.

The numerical simulations use the length scale $r_0$ and time scale $1/\omega_0$, where

$$\omega_0^2 = \frac{e}{m}\frac{E_0}{r_0} = \frac{1}{4\pi\epsilon_0}\frac{Ze^2}{mr_0^3}, \tag{9}$$

(setting $q = Ze$). When converting to dimensionless positions and times, it is convenient to make replacement $c \to r_0\omega_0/\eta$. Consider, for example, the energy function given by

$$\mathcal{E}(v)/mc^2 = \gamma\left(\frac{1-vu_x/c^2}{\sqrt{1-u^2/c^2}}\right) - \frac{Ze^2}{4\pi\epsilon_0 mc^2}\frac{1}{\tilde{r}} = \gamma\left(\frac{1-\eta^2(vu_x)/(r_0\omega_0)^2}{1-\eta^2u^2/(r_0\omega_0)^2}\right) - \eta^2\frac{r_0}{\tilde{r}}.$$

## II. COMPUTER CODES

The MATLAB computer codes include the following:

- orbit_constV.m
- orbit_accelV.m
- calc_ret_time_accelV.m
- calc_fields_accelV.m

The first script, orbit_constV.m, numerically calculates the orbits for a nucleus in uniform motion, as discussed in Sec. IV of the text. The second script, orbit_accelV.m, numerically calculates the orbits for a nucleus with the trajectory described above, and as discussed in Sec. V of the text.. This second script uses two functions. The first function, calc_ret_time_accelV.m, calculates the retarded time $t_r$, as well as $x_n$, $v$, and $a$. These are then used in the second function, calc_fields_accelV.m, to calculate the fields $E_x$, $E_y$, and $B_z$.
